# Supplementary material for: Origins and Nature of Macroeconomic Instability in Vector Autoregressions
Source: arXiv:2512.20152 source file (2025-12-23)
Supplement: Supplementary file 1 [file part_appendix_model.tex]

%% -------------------------------------------------------------------------- %%
%% -------------------------------------------------------------------------- %%

\newpage
\section{Factor-TVP-VAR: Estimation Details}
\label{appsec_model}

\colDO{draft2019: Appendices A.1 and A.2 }

%% -------------------------------------------------------------------------- %%
%% -------------------------------------------------------------------------- %%
